# Supplementary material for: Null-text Inversion for Editing Real Images using Guided Diffusion Models
Source: arXiv:2211.09794 source file (2022-11-17)
Supplement: Supplementary file 1 [file ours_supp.tex]

\begin{figure}
\setlength{\tabcolsep}{0.5pt}
    %\centering
    { \scriptsize %\footnotesize

\begin{tabular}{p{0.25\columnwidth} @{\hskip 0.04in} p{0.25\columnwidth} p{0.25\columnwidth} p{0.25\columnwidth}}

\multicolumn{4}{c}{"A living room with a couch and pillows"} \\

{\includegraphics[width=0.25\columnwidth]{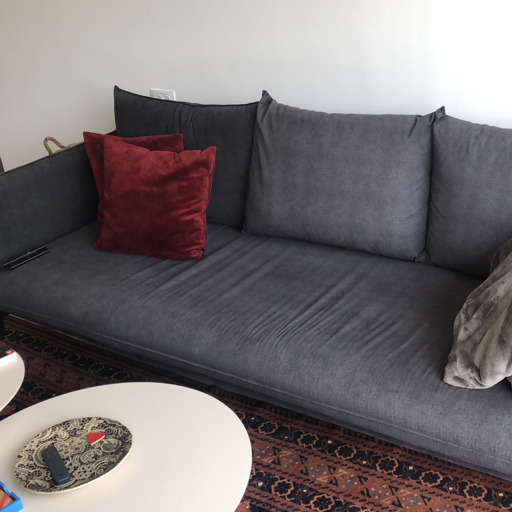}}&
{\includegraphics[width=0.25\columnwidth]{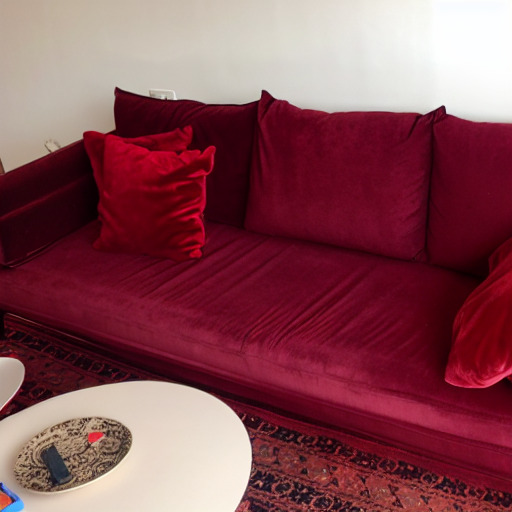}} &
{\includegraphics[width=0.25\columnwidth]{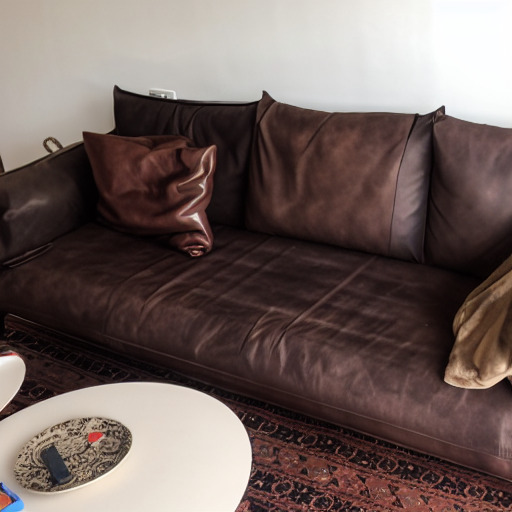}} &
{\includegraphics[width=0.25\columnwidth]{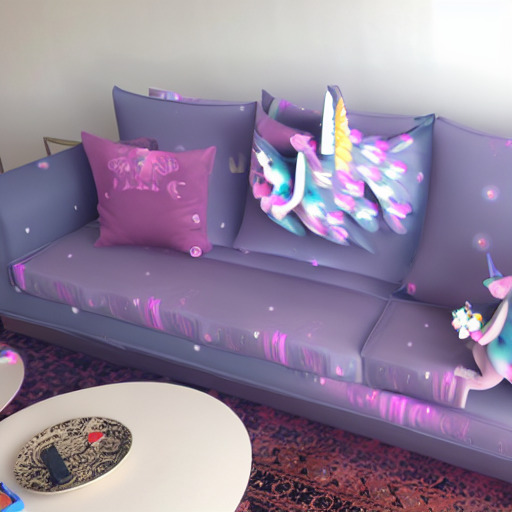}} \\

\multicolumn{1}{c}{Input}&
"{\color{RoyalPurple} \bf red velvet~~~~~} couch..." &
"{\color{RoyalPurple} \bf leather} couch..." &
"{\color{RoyalPurple} \bf unicorn pattern} couch..." \\

\midrule
\multicolumn{4}{c}{"A basket with apples on a chair"} \\

{\includegraphics[width=0.25\columnwidth]{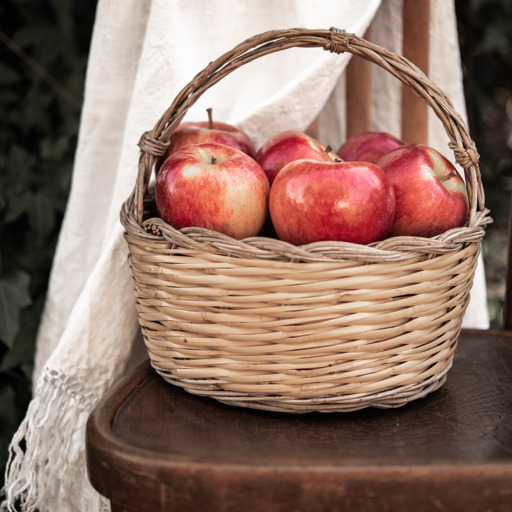}} &
{\includegraphics[width=0.25\columnwidth]{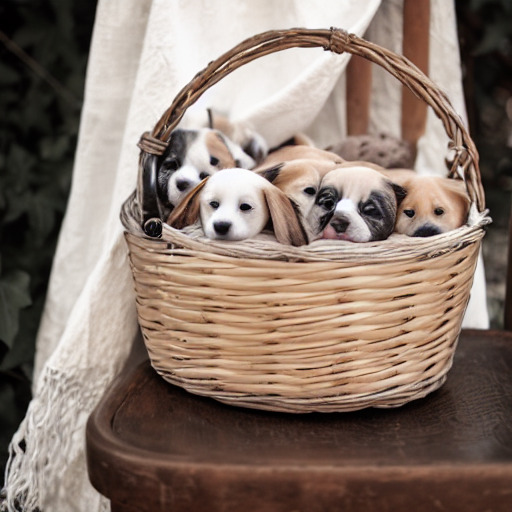}} &
{\includegraphics[width=0.25\columnwidth]{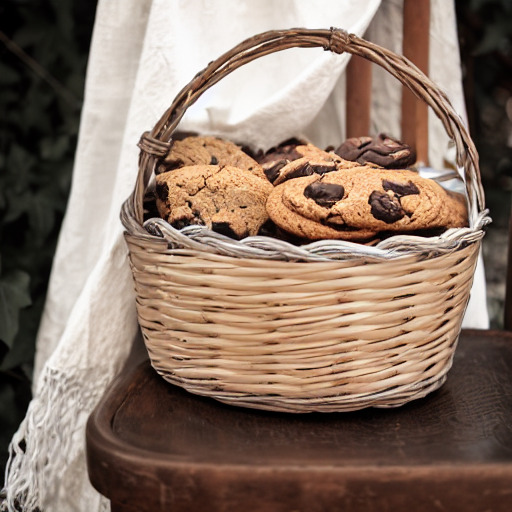}} &
{\includegraphics[width=0.25\columnwidth]{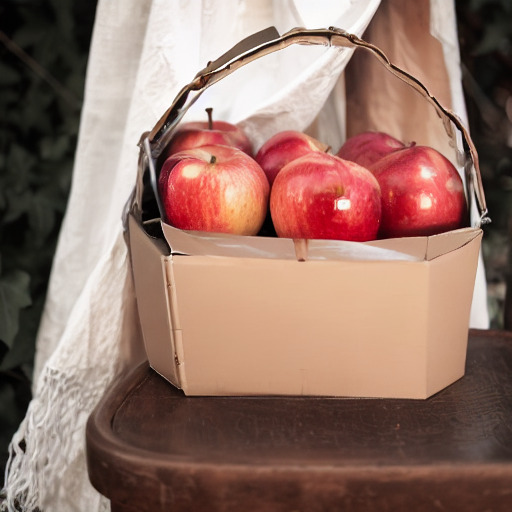}} \\

\multicolumn{1}{c}{Input}&
"apples"$\rightarrow$ "{\color{RoyalPurple}\bf puppies}" &
"apples"$\rightarrow$ "{\color{RoyalPurple} \bf cookies}" &
"{\color{RoyalPurple} \bf cardboard} basket..." \\

% \midrule
% \multicolumn{4}{c}{"A child is climbing on a tree"} \\

% {\includegraphics[width=0.25\columnwidth]{images/gt/kid_tree.jpg}} &
% {\includegraphics[width=0.25\columnwidth]{images/ours/kid_tree_097.jpg}} &
% {\includegraphics[width=0.25\columnwidth]{images/ours/kid_tree_098.jpg}} &
% {\includegraphics[width=0.25\columnwidth]{images/ours/kid_tree_099.jpg}} \\

% \multicolumn{1}{c}{Input}&
% "child"$\rightarrow$ "{\color{RoyalPurple} \bf tiger}" &
% "child"$\rightarrow$ "{\color{RoyalPurple} \bf zebra}" &
% "child"$\rightarrow$ "{\color{RoyalPurple} \bf monkey}" \\

\midrule
\multicolumn{4}{c}{"A girl sitting on the grass and holding a ball"} \\

{\includegraphics[width=0.25\columnwidth]{images/gt/girl_ball_058.jpg}} &
{\includegraphics[width=0.25\columnwidth]{images/ours/ball_057.jpg}} &
{\includegraphics[width=0.25\columnwidth]{images/ours/ball_064.jpg}} &
{\includegraphics[width=0.25\columnwidth]{images/ours/ball_065.jpg}} \\

\multicolumn{1}{c}{Input}&
"{\color{RoyalPurple} \bf golden} ball..." &
"girl"$\rightarrow$ "{\color{RoyalPurple} \bf tiger}" &
"girl"$\rightarrow$ "{\color{RoyalPurple} \bf dog}" \\

% \midrule
% \multicolumn{4}{c}{"A bicycle is parking on the side of the street"} \\

% {\includegraphics[width=0.25\columnwidth]{images/gt/bicycle_039.jpg}} &
% {\includegraphics[width=0.25\columnwidth]{images/ours/bicycle_039.jpg}} &
% {\includegraphics[width=0.25\columnwidth]{images/ours/bicycle_044.jpg}} &
% {\includegraphics[width=0.25\columnwidth]{images/ours/bicycle_047.jpg}} \\

% \multicolumn{1}{c}{Input}&
% "{\color{RoyalPurple} \bf blue} bicycle" &
% "{\color{RoyalPurple} \bf snowy} street" &
% "street"$\rightarrow$ "{\color{RoyalPurple} \bf forest}"\\

\midrule
\multicolumn{4}{c}{"two birds sitting on a branch"} \\

{\includegraphics[width=0.25\columnwidth]{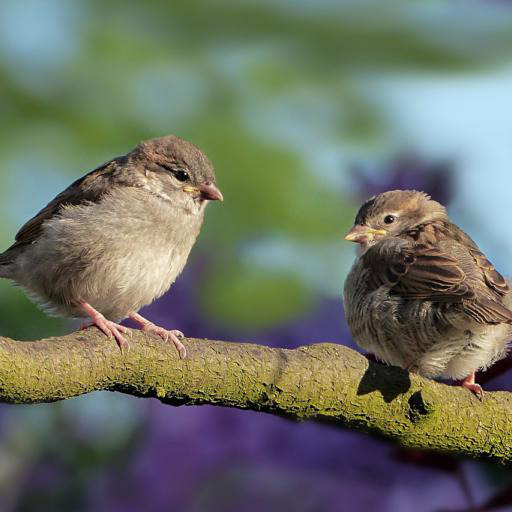}} &
{\includegraphics[width=0.25\columnwidth]{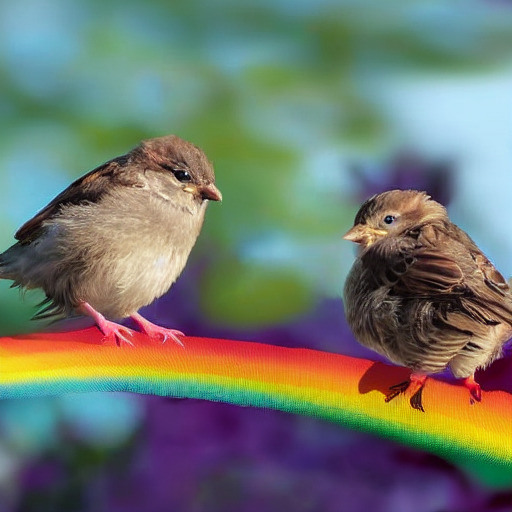}} &
{\includegraphics[width=0.25\columnwidth]{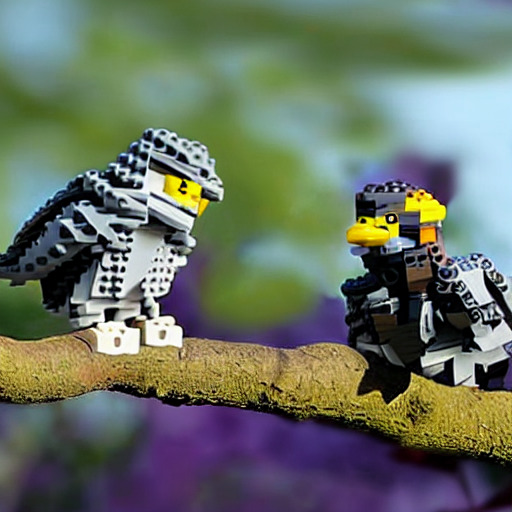}} &
{\includegraphics[width=0.25\columnwidth]{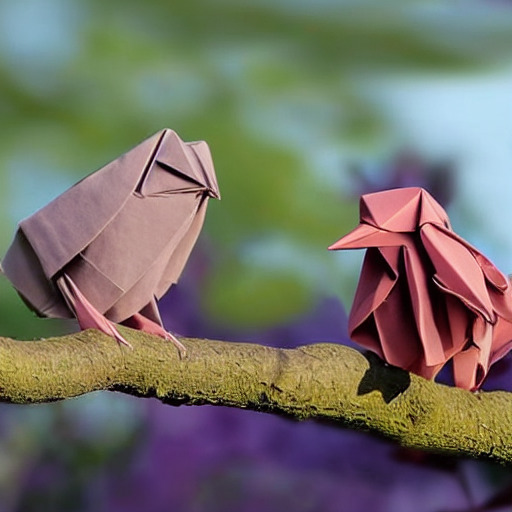}} \\

\multicolumn{1}{c}{Input}&
"branch"$\rightarrow$ "{\color{RoyalPurple} \bf rainbow}" &
"{\color{RoyalPurple} \bf lego} birds..." &
"{\color{RoyalPurple} \bf origami} birds..." \\

\end{tabular}
}

\caption{{\bf Real image editing using our method.} {\it We first apply our NULL-text inversion over the real input images, achieving near-perfect reconstruction. Then, Prompt-to-Prompt text-based editing is applied. As can be seen, our inversion scheme provide high-fidelity while retaining high editability. See additional examples in the supplementary materials. } }
% \vspace{-0.15cm}
% \ron{The gap is best viewed in the supplementary videos.}}
\label{fig:comparison} %\vspace{-7pt}
\end{figure}
